# Supplementary material for: SP2Bench: A SPARQL Performance Benchmark
Source: arXiv:0806.4627 source file (2008-10-21)
Supplement: Supplementary file 1 [file appendix.tex]

\section{Attribute Distribution (full table)}
\begin{table*}[h]
\begin{center}
{\footnotesize
\begin{tabular}{l||c|c|c|c|c|c|c|c}
&
\begin{turn}{90}article\end{turn} &
\begin{turn}{90}inproceedings\end{turn} &
\begin{turn}{90}proceedings\end{turn} &
\begin{turn}{90}book\end{turn} &
\begin{turn}{90}incollection\end{turn} &
\begin{turn}{90}phdthesis\end{turn} &
\begin{turn}{90}mastersthesis\end{turn} &
\begin{turn}{90}www\end{turn}\\
\hline
\hline
address & 0.0000	& 0.0000 & 0.0004 & 0.0000 & 0.0000	& 0.0000 & 0.0000 & 0.0000

\\
\hline
author & 0.9888	& 0.9969 & 0.0001 & 0.8993	& 0.9946 & 1.0000	& 1.0000 & 0.9972
\\
\hline
booktitle & 0.0006 & 1.0000	& 0.9564 & 0.0153 & 1.0000 & 0.0000 & 0.0000 & 0.0001
\\
\hline
cdrom & 0.0123 & 0.0170	& 0.0000 & 0.0032 & 0.0206 & 0.0000	& 0.0000 & 0.0000
\\
\hline
chapter & 0.0000 & 0.0000 & 0.0000 & 0.0000 & 0.0008 & 0.0000 & 0.0000 & 0.0000
\\
\hline
cite & 0.0052 & 0.0109 & 0.0001 & 0.0081 & 0.0070 & 0.0000 & 0.0000 & 0.0000
\\
\hline
crossref & 0.0007 & 0.7882 & 0.0015 & 0.0000 & 0.5010 & 0.0000 & 0.0000 & 0.0000
\\
\hline
editor & 0.0000 & 0.0000 & 0.7971 & 0.0983 & 0.0000 & 0.0000 & 0.0000 & 0.0004
\\
\hline
ee & 0.6462 & 0.6442 & 0.0020 & 0.0081 & 0.0463 & 0.1348 & 0.0000 & 0.0000
\\
\hline
isbn & 0.0000 & 0.0000 & 0.8634 & 0.9283 & 0.0109 & 0.0225 & 0.0000 & 0.0000
\\
\hline
journal & 0.9994 & 0.0000 & 0.0004 & 0.0000 & 0.0000 & 0.0000 & 0.0000 & 0.0000
\\
\hline
month & 0.0071 & 0.0000 & 0.0001 & 0.0008 & 0.0000 & 0.0337 & 0.0000 & 0.0000
\\
\hline
note & 0.0000	& 0.0000 & 0.0002 & 0.0000 & 0.0000 & 0.0000 & 0.0000 & 0.0244
\\
\hline
number & 0.9347 & 0.0001 & 0.0010 & 0.0000 & 0.0000 & 0.0337 & 0.0000 & 0.0000
\\
\hline
page & 0.9404	& 0.9502 & 0.0000 & 0.0000 & 0.9922 & 0.0000 & 0.0000 & 0.0000
\\
\hline
publisher & 0.0007 & 0.0000 & 0.9733 & 0.9992 & 0.0354 & 0.0449 & 0.0000 & 0.0000
\\
\hline
school & 0.0000 & 0.0000 & 0.0000 & 0.0000 & 0.0000 & 1.0000 & 1.0000 & 0.0000
\\
\hline
series & 0.0000	& 0.0000 & 0.5812 & 0.5375 & 0.0000 & 0.0225 & 0.0000 & 0.0000
\\
\hline
title & 1.0000 & 1.0000 & 1.0000 & 1.0000 & 1.0000 & 1.0000 & 1.0000 & 1.0000
\\
\hline
url & 0.9984 & 1.0000 & 0.9859 & 0.2256 & 0.9988 & 0.0225 & 0.3750 & 0.9647
\\
\hline
volume & 0.9980 & 0.0000 & 0.5690 & 0.5068 & 0.0000 & 0.0112 & 0.0000 & 0.0000
\\
\hline
year & 1.0000 & 1.0000 & 1.0000 & 1.0000 & 1.0000 & 1.0000 & 1.0000 & 0.0012
\end{tabular}
}
\end{center}
\caption{Attribute Probability Distribution.}
\label{tbl:attributes_full}
\end{table*}
